# Supplementary material for: Delayed Geometric Discounts: An Alternative Criterion for Reinforcement Learning
Source: arXiv:2209.12483 source file (2022-09-26)
Supplement: Supplementary file 1 [file algorithms.tex]

\section{Algorithms}
    In this section we properly introduce the algorithms
